# Supplementary material for: Combinatorial Bandits under Strategic Manipulations
Source: arXiv:2102.12722 source file (2021-11-19)
Supplement: Supplementary file 1 [file appendix.tex]

\section{Regret analysis of strategic UCB}

\begin{namedtheorem}[Lemma \ref{lambda} (Re-statement)]
Let $\Lambda_{i,t} = \sqrt{\frac{3 \log{t} }{2K_{i,t-1}}} + \frac{\rho_{i,t-1}}{K_{i,t-1}}$% + \frac{B_{max}}{K_{i,t-1}}$
, where $\rho_{i,t-1}$ is the total strategic budget spent by arm $i$ up to time $t-1$ and $K_{i,t-1}$ be the total number of pulls of arm $i$ up to time $t-1$. Define the event $E_t = \{  |\ \widetilde{\mu}_{i,t-1} - \mu_{i}| \leq \Lambda_{i,t}, \forall i \in [m]\}$, where $\mu_i$ is the true mean of arm $i$'s underlying distribution. 
%The probability of event $E_t$ is bounded when $K_{i,t-1} > \psi_t$, $\psi_t = \frac{8B_{max}\cdot f^{-1}(\Delta_{min}) + 6\log{T}} {\left[f^{-1}(\Delta_{min})\right]^2}$%
Then, $\mathbb{P}(\lnot E_t)\leq 2m \cdot t^{-2}$.
\end{namedtheorem}

\begin{proof}
Denote $\hat{\mu}_{i,t-1} = \frac{\sum_{j=1}^{t-1} x_{i,j}}{K_{i,t-1}}$ as the estimation of the expected reward without the manipulated variable $z_{i,t}$. By the definition of $\hat{\mu}_{i,t}$ and $\widetilde{\mu}_{i,t}$,
\begin{align}
& \mathbb{P}\left(|\widetilde{\mu}_{i,t-1} - \mu_i| > \sqrt{\frac{3\log{t}}{2K_{i,t-1}}} + \frac{\rho_{i,t-1}}{K_{i,t-1}}\right) \notag \\
    =\ & \mathbb{P}\left(\left|\hat{\mu}_{i,t-1} + \frac{\rho_{i,t-1}}{K_{i,t-1}}- \mu_i\right| > \sqrt{\frac{3\log{t}}{2K_{i,t-1}}} + \frac{\rho_{i,t-1}}{K_{i,t-1}} \ \right) \notag \\
    =\ & \mathbb{P}\left(\hat{\mu}_{i,t-1} - \mu_i > \sqrt{\frac{3\log{t}}{2K_{i,t-1}}}  \ \right) + \mathbb{P}\left(\hat{\mu}_{i,t-1} - \mu_i < -\sqrt{\frac{3\log{t}}{2K_{i,t-1}}} -2 \frac{\rho_{i,t-1}}{K_{i,t-1}}  \right) \notag \\
    \leq\ & \mathbb{P}\left(\hat{\mu}_{i,t-1} - \mu_i > \sqrt{\frac{3\log{t}}{2K_{i,t-1}}} \ \right) + \mathbb{P}\left(\hat{\mu}_{i,t-1} - \mu_i <  -\sqrt{\frac{3\log{t}}{2K_{i,t-1}}}\right) \notag \\
    =\ & \sum_{s=1}^{t-1} \mathbb{P}\left(|\hat{\mu}_{i,t-1} - \mu_i|> \sqrt{\frac{3\log{t}}{2s}}, K_{i,t-1} = s \ \right) \notag \\
    \leq\ & \sum_{s=1}^{t-1} \mathbb{P}\left(|\hat{\mu}_{i,{t-1}} - \mu_i|  > \sqrt{\frac{3\log{t}}{2s}}\ \right)\notag\\
    \leq\ & 2t\cdot \exp{(-3\log{t})} = \frac{2}{t^2} \,, \nonumber
\end{align}
where the last inequality follows the Chernoff-Hoeffding bound. By the union bound,
\[
\quad \mathbb{P}(\lnot E_t) = \mathbb{P}\left( \{   |\widetilde{\mu}_{i,t-1} - \mu_{i}| > \Lambda_{i,t}, \forall i \in [m]\} \right)\leq 2m \cdot t^{-2} \,. \qedhere
\]
\end{proof}

\begin{namedtheorem}[Theorem \ref{appendixA} (Re-statement)]
The regret of the strategic CUCB algorithm with m strategic arms in time horizon $T$ using an $(\alpha,\beta)$-approximation oracle is at most 
\begin{align}
 m\cdot\Delta_{max}\left( \frac{8B_{max} f^{-1}(\Delta_{min}) + 6\log{T}} {\left(f^{-1}(\Delta_{min})\right)^2} + \frac{\pi^2}{3}+1 \right)\,, \notag \nonumber
\end{align}
where $f^{-1}(\cdot)$ is the inverse bounded smoothness function.
\end{namedtheorem}

\begin{proof}
We start by introducing a few notations. Let $F_t$ to be the event where the $(\alpha,\beta)$-approximation oracle fails to produce an $\alpha$-approximation answer with respect to the input  $\bm{\Bar{\mu}} = (\Bar{\mu}_{1,t},\Bar{\mu}_{2,t},.....,\Bar{\mu}_{m,t})$ at time $t$. By definition of a $(\alpha,\beta)$-approximation oracle, we have $\mathbb{P}(F_t) \leq 1 - \beta$. Observe that at an arbitrary time $t$, a suboptimal arm subset may be selected due to two reasons, i) the $(\alpha, \beta)$-approximation oracle fails to provide an $\alpha$-approximate arm subset with respect to the input vector $\bm{\Bar{\mu}} = (\Bar{\mu}_{1,t},\Bar{\mu}_{2,t},.....,\Bar{\mu}_{m,t})$ and ii) the estimated mean vector $\bm{\bar{\mu}} = (\bar{\mu}_{1,t}, \bar{\mu}_{2,t},......,\bar{\mu}_{m,t})$ deviates from true values by a significant amount. 

To account for $\sum^T_{t=1} \mathbb{I}(S_t \in S_B)$,where $\mathbb{I}(S_t \in S_B)$ is 1 when algorithm choose a suboptimal arm subset, $S_t \in S_B$, at time $t$, we introduce a counter $N_i$ for each arm $i\in[m]$ after the $m$-round initialization and let $N_{i,t}$ be the value of $N_i$ at time $t$. We initialize $N_{i,m} = 1$. By definition, $\sum_{i \in [m]} N_{i,m} = m$. For $t > m$, the counter $N_{i,t}$ is updated as follows.
\begin{itemize}
    \item If $S_t \in S_B$, then $N_{{i'},t} = N_{{i'},t-1} + 1$ where $i' = \argmin_{i \in S_t} N_{i,t-1}$. In the case that $i'$ is not unique, we break ties arbitrarily.
    \item If $S_t \not \in S_B$, no counters will be updated then. 
\end{itemize}  
As such, the total number of pulls of suboptimal arm subsets is less than or equal to $\sum_{i=1}^m N_{i,T}$.

Define $\psi_t = \frac{8B_{max} f^{-1}(\Delta_{min}) + 6\log{t}} {\left(f^{-1}(\Delta_{min})\right)^2} > c\,, $
where $c$ is the larger solution of the following equation, 
\begin{align}
    &\frac{\left(f^{-1}(\Delta_{min})\right)^2}{4} c^2 
    - \left(2B_{max} f^{-1}(\Delta_{min}) + \frac{3\log{t}}{2}\right)c + 4B_{max}^2 = 0\,. \label{square}
\end{align}
By solving Equation \eqref{square}, we have  
\begin{align}
    c &= \frac{2\left(2B_{max} f^{-1}(\Delta_{min}) + \frac{3\log{t}}{2}\right)} {\left(f^{-1}(\Delta_{min})\right)^2} + \frac{2\sqrt{\left(2B_{max} f^{-1}(\Delta_{min}) + \frac{3\log{t}}{2}\right)^2 -4(f^{-1}(\Delta_{min})) B_{max}}} {\left(f^{-1}(\Delta_{min})\right)^2}\,. \label{psi}
\end{align}

%Later we will explain why we design $\psi_t$ and $c$ in this subtle way. 
We then decompose the total number $\sum_{i=1}^m N_{i,T}$ of pulls of suboptimal arm subsets as
\begin{align}
\quad\sum_{i=1}^m N_{i,T} =\ & m +\sum_{t=m+1}^T \mathbb{I}\{ S_t \in S_B\} \notag \\
 =\ & m +\sum_{t=m+1}^T \sum_{i\in[m]}^m \mathbb{I}\{ S_t \in S_B, N_{i,t} > N_{i,t-1}, N_{i,t-1} \leq \psi_t\} \notag \\
& + \sum_{t=m+1}^T \sum_{i\in[m]}^m \mathbb{I}\{ S_t \in S_B, N_{i,t} > N_{i,t-1}, N_{i,t-1} > \psi_t\}\notag \\
 \leq\ & m + m\psi_T +\sum_{t=m+1}^T \sum_{i\in[m]}^m \mathbb{I}\{ S_t \in S_B, N_{i,t} > N_{i,t-1}, N_{i,t-1} > \psi_t\}\notag \\
 =\ & m + m\psi_T+\sum_{t=m+1}^T \mathbb{I}\{  S_t \in S_B , \forall i \in S_t, N_{i,t-1} > \psi_t\} \,.\label{8}
\end{align}

The first inequality follows as $\sum_{t=m+1}^T \mathbb{I}\{ S_t \in S_B, \forall i \in S_t, N_{i,t-1} \leq \psi_t\}$ can be trivially upper bounded by $\psi_t$ and the second equality holds by our rule of updating the counters. 

The third term of Equation \eqref{8} can be further decomposed according to whether the oracle fails, 
\begin{align}
&\quad \sum_{t=m+1}^T \mathbb{I}\{ S_t \in S_B,  N_{i,t-1} > \psi_t, \forall i \in S_t\}\notag\\
&\leq \sum_{t=m+1}^T (\mathbb{I}\{F_t\} + \mathbb{I}\{ \lnot F_t, S_t \in S_B,  K_{i,t-1} > \psi_t, \forall i \in S_t\})\label{ke} \\
&= (T-m)(1-\beta)+\sum_{t=m+1}^T \mathbb{I}\{ \lnot F_t, S_t \in S_B, K_{i,t-1} > \psi_t , \forall i \in S_t\}\,. \notag
\end{align}
 %We then bound $\sum_{t=m+1}^T \mathbb{I}\{ \lnot F_t, S_t \in S_B,\forall i \in S_t,K_{i,t-1} > \psi_t\}$. 

Let $\Lambda_{i,t} = \sqrt{\frac{3 \log{t} }{2K_{i,t-1}}} + \frac{\rho_{i,t-1}}{K_{i,t-1}}$ where $\rho_{i,t-1}$ is the total strategic budget spent by arm $i$ up to time $t-1$. Define event $E_t = \{  |\ \widetilde{\mu}_{i,t-1} - \mu_{i}| \leq \Lambda_{i,t}, \forall i \in [m]\}$, where $\mu_i$ is the true mean of arm $i$'s underlying distribution without manipulation. We continue the proof under $\mathbb{P}(\{ E_t, \lnot F_t, S_t \in S_B, K_{i,t-1} > \psi_t, \forall i \in S_t \}) = 0$ and prove it afterwards.

Since $\mathbb{P}\left(\{ E_t, \lnot F_t, S_t \in S_B, K_{i,t-1} > \psi_t , \forall i \in S_t\} \right) = 0$, by inclusion-exclusion principle, 
$ \mathbb{P}(\{\lnot F_t, S_t \in S_B, K_{i,t-1} > \psi_t, \forall i \in S_t\}) \leq \mathbb{P}(\lnot E_t)\,.$ Denote $\hat{\mu}_{i,t-1} = \frac{\sum_{j=1}^{t-1} x_{i,j}}{K_{i,t-1}}$ as the estimation of the expected reward without the manipulated variable $z_{i,t}$. By the definition of $\hat{\mu}_{i,t}$ and $\widetilde{\mu}_{i,t-1}$,
\begin{align}
&\quad \mathbb{P}\left(|\widetilde{\mu}_{i,t-1} - \mu_i| > \sqrt{\frac{3\log{t}}{2K_{i,t-1}}} + \frac{\rho_{i,t-1}}{K_{i,t-1}} +  \frac{B_{max}}{K_{i,t-1}}  \ \right) \notag \notag \\
    &= \mathbb{P}\left(\left|\hat{\mu}_{i,t-1} + \frac{\rho_{i,t-1}}{K_{i,t-1}}- \mu_i\right| > \sqrt{\frac{3\log{t}}{2K_{i,t-1}}} + \frac{\rho_{i,t-1}}{K_{i,t-1}}+\frac{B_{max}}{K_{i,t-1}} \right) \notag \\
    &\leq \mathbb{P}\left(\left|\hat{\mu}_{i,t-1} + \frac{\rho_{i,t-1}}{K_{i,t-1}}- \mu_i\right| > \sqrt{\frac{3\log{t}}{2K_{i,t-1}}} + \frac{\rho_{i,t-1}}{K_{i,t-1}} \ \right) \notag \\
    &\leq 2t^{-2}\,,
\end{align}
where the last inequality holds due to Lemma \ref{lambda}.

By the union bound, 
\begin{align}
    &\ \quad \mathbb{P}(\lnot E_t) = \mathbb{P}(  \{  |\widetilde{\mu}_{i,t-1} - \mu_{i}| > \Lambda_{i,t}, \forall i \in [m] \} \ ) \leq 2m \cdot t^{-2}\,. \notag
\end{align}
Hence, 
\begin{align}
     \mathbb{P}(\{\lnot F_t, S_t \in S_B,  \forall i \in S_t, K_{i,t-1} > \psi_t, \forall i \in S_t\}) \leq \mathbb{P}(\lnot E_t) \leq 2m \cdot t^{-2}\,. \notag
\end{align}

We now show that $\mathbb{P}(\{ E_t, \lnot F_t, S_t \in S_B, K_{i,t-1} > \psi_t, \forall i \in S_t \}) = 0$. Let $\Lambda = \sqrt{\frac{3 \log{t}}{2\psi_t}}+ \frac{2B_{max}}{\psi_t} $, which is not a random variable, and $B_{max} = max_{i \in [m]} B_i$, where $B_i$ is the strategic budget for arm $i$. For variable $\Lambda_{i,t}$, let $\Lambda_{i,t}^{\ast} = \max \{\Lambda_{i,t}\}$. Since $K_{i,t-1} > \psi_t$ and $B_{max} \geq B_i \geq \rho_i$, we have $\Lambda > \Lambda_{i,t}^{\ast}$.  According to line 7 of Algorithm 1, we have $\Bar{\mu}_{i,t}= \widetilde{\mu}_{i,t-1} + \sqrt{\frac{ 3 \log{t} }{2K_{i,t-1}}} + \frac{B_{max}}{K_{i,t-1}}$ and $\bar{\mu}_{i,t} = \hat{\mu}_{i,t-1} + \frac{\rho_{i,t-1}}{K_{i,t-1}} + \sqrt{\frac{ 3 \log{t} }{2K_{i,t-1}}}+ \frac{B_{max}}{K_{i,t-1}}$. Thus,  $|\hat{\mu}_{i,t-1} - \mu_i| \leq \Lambda_{i,t}$ implies that $0 < \bar{\mu}_{i,t-1} - \mu_i \leq 2\Lambda_{i,t} \leq 2\Lambda_{i,t}^{\ast} \leq 2\Lambda$, for $ i \in S_t$.

Recall $S^{\ast} = \argmax_{S \in \mathcal{S}} r_{\bm{\mu}}(S)$ and ${OPT}_{\bm{\mu}} = \max_{S\in \mathcal{S}} r_{\bm{\mu}}(S)$. Suppose $\{E_t, \lnot F_t, S_t \in S_B, \forall i \in S_t, K_{i,t-1} > \psi_t \} $ happens at time $t$, the following holds
\begin{align}
    \quad r_{\bm{\mu}}(S_t) + f(2\Lambda) \notag & \geq r_{\bm{\mu}}(S_t) + f(2\Lambda_{i,t}^{\ast})  \geq r_{\bm{\bar{\mu}}}(S_t) \\ \notag
    & \geq \alpha \cdot {OPT}_{\bar{\bm{\mu}}}\geq \alpha \cdot r_{\bar{\bm{\mu}}}(S^{\ast}_{\bm{\mu}}) \geq \alpha \cdot r_{{\bm{\mu}}} (S^{\ast}_{\bm{\mu}}) \\ \notag
    & = \alpha \cdot {OPT}_{\bm{\mu}}\,. \notag
\end{align} 
The first inequality is due to the strict monotonicity of $f(\cdot)$ and $\Lambda > \Lambda_{i,t}^{\ast}$. The second inequality is due to the bounded smoothness property and $|\bar{\mu}_{i,t-1} - \mu_i | \leq 2\Lambda_{i,t}$. The third inequality is due to the fact that $\lnot F_t$ implies $S_t \geq \alpha \cdot opt_{\bm{\mu}}$. The forth inequality is by the definition of $opt_{\bm{\mu}}$. The last inequality is is due to the monotonicity of $r_{\bm{\mu}}(S)$ and $0 < \bar{\mu}_{i,t-1} - \mu_i$. 

Let $\kappa = \sqrt{\frac{3 \log{t}}{2c}} + \frac{2B_{max}}{c}$ where $c$ takes the value defined in Equation \eqref{square}. Given $\psi_t > c$, we have $\Lambda = \sqrt{\frac{3 \log{t}}{2\psi_t}} + \frac{2B_{max}}{\psi_t} < \kappa$. By Equation \eqref{psi}, we have $f(2\Lambda) < f(2\kappa) = \Delta_{min}$ and $\Delta_{min} > \alpha \cdot opt_{\bm{\mu}} -  r_{\bm{\mu}}(S_t)$, which contradicts the definition of $\Delta_{min}$ and the fact that $S_t \in S_B$. Therefore,
\begin{equation}
     \mathbb{P}(E_t, \lnot F_t, S_t \in S_B, \forall i \in S_t, K_{i,t-1} > \psi_t )= 0\,. \notag
\end{equation}
%Now that we have upper bounded each of the decomposed term of $\mathbb{E}\left[\sum_{i=1}^m N_{i,T} \right]$, we are ready to derive our final regret bound. 
Based on the above analysis, we can upper bound the total number of suboptimal pulls as 
\begin{align}
     \mathbb{E}\left[\sum_{i=1}^m N_{i,T} \right] 
     &\leq m(1+\psi_T) + (T-m)(1-\beta) + \sum_{t=m+1}^T \frac{2m}{t^2}\notag \\
    &= m\left(1+\frac{8B_{max} f^{-1}(\Delta_{min}) + 6\log{T}} {\left(f^{-1}(\Delta_{min})\right)^2}\right) + (T-m)(1-\beta) + \sum_{t=m+1}^T \frac{2m}{t^2}\,.
\end{align}
Since the cumulative regret relate closely to the total number of suboptimal pulls $\mathbb{E}[\sum_{i=1}^m N_{i,T}]$, the upper bound of cumulative regret is thus
\begin{align}
    \quad Regret_{\bm{\mu},\alpha,\beta}(T)
    \leq\ &  T \cdot \alpha  \beta  \text{OPT}_{\bm{\mu}} - \left( T \cdot \alpha  \text{OPT}_{\bm{\mu}} - \mathbb{E} \left[ \sum_{i=1}^m N_{i,T} \right] \Delta_{max} \right)
    \notag \\
     =\ & (\beta-1) T \cdot \alpha \text{OPT}_{\bm{\mu}}  + \Delta_{max}\left( m \left(1+\frac{8B_{max} f^{-1}(\Delta_{min}) + 6\log{T}}  {\left(f^{-1}(\Delta_{min})\right)^2}\right)\notag \right) \notag \\
     &+ \Delta_{max}\left((T-m)  (1-\beta)  +\sum_{t=m+1}^T \frac{2m}{t^2}\right)\notag\\
     \leq\ &  ((T-m) \cdot \Delta_{max}- T \cdot \alpha \text{OPT}_{\bm{\mu}})(1-\beta)
      \notag \\
     & + m \cdot \Delta_{max}\left(1+\frac{8B_{max} f^{-1}(\Delta_{min}) + 6\log{T}} {\left(f^{-1}(\Delta_{min})\right)^2} + \frac{\pi^2}{3}\right)\,.\notag
\end{align}
Each time the algorithm pull a suboptimal arm subset $S_t \in S_B$ at time $t$, the algorithm incur an additional regret of at most $\Delta_{max}$, which is less than or equal to $\alpha \cdot opt_{\bm{\mu}}$. Thus,
\begin{align}
    &\quad (T-m) \Delta_{max}-T\alpha \cdot \text{OPT}_{\bm{\mu}} \notag\\
    &\leq (T-m) \alpha \cdot \text{OPT}_{\bm{\mu}}- T\alpha\cdot \text{OPT}_{\bm{\mu}}\notag\\
    &=-m  \alpha\cdot \text{OPT}_{\bm{\mu}} < 0\,.\notag
\end{align}
As a result, the regret of the strategic CUCB algorithm under strategic manipulations of reward is at most
\begin{align}
    &Regret_{\bm{\mu},\alpha,\beta}(T)\leq m \cdot \Delta_{max} \left(\frac{8B_{max} f^{-1}(\Delta_{min}) + 6\log{T}} {\left(f^{-1}(\Delta_{min})\right)^2} + \frac{\pi^2}{3} + 1\right)\notag \,. \qedhere
\end{align}
\end{proof}

\section{Lower bound on the strategic budget}
\begin{namedtheorem}[Theorem \ref{lower}]
In stochastic multi-armed bandit problems, for a strategic suboptimal arm $i$, under time horizon $T$ and without access to other arms' information, the minimum strategic budget needed for it to be pulled $\omega(\log{T})$ is $\omega(\log{T})$. The regret incurred for any bandits learning algorithm is thus $\omega(\log{T})$.
\end{namedtheorem}
\begin{proof}
Let time $t \in [1,T]$ be the time step arm $i$ is last pulled under UCB algorithm and $\eta$ is a parameter chosen by the algorithm. The following inequality must stands at time $t$,
\begin{align*}
& \hat{\mu}_{i,t} + \sqrt{\frac{2\log(K_{i,t}^2/\eta^2)}{K_{i,t}}} + \frac{\rho_i}{K_{i,t}}\geq \hat{\mu}_{i^{\ast},t} + \sqrt{\frac{2\log(K_{i^{\ast},t}^2/\eta^2)}{K_{i^{\ast},t}}}\,.
\end{align*}
By the Chernoff-Hoeffding bound and the union bound, 
\begin{align*}
&\quad \mathbb{P} \left(\hat{\mu}_{i,t}  - \mu_i  \geq \sqrt{\frac{2\log(K_{i,t}^2/\eta^2)}{K_{i,t}}}\right)\\
&\leq \sum^{t}_{s=1} \mathbb{P}  \left( \hat{\mu}_{i,t}  - \mu_i  \geq \sqrt{\frac{2\log(s^2/\eta^2)}{s}}, K_{i,t} = s \right) \\
&\leq\sum^{t}_{s=1} \mathbb{P}  \left( \hat{\mu}_{i,t}  - \mu_i  \geq \sqrt{\frac{2\log(s^2/\eta^2)}{s}}\right) \\
& \leq \sum^{t}_{s=1} \frac{\eta^2}{s^2} = \eta^2\sum^{t}_{s=1} \frac{1}{s^2} \leq  \frac{\pi^2}{6} \eta^2 \,.
\end{align*}
Thus $\hat{\mu}_{i,t}  - \mu_i  \leq \sqrt{\frac{2\log(K_{i,t}^2/\eta^2)}{K_{i,t}}}$ and similarly $\mu_{i^{\ast},t} -  \hat{\mu}_{i^{\ast}}  \leq \sqrt{\frac{2\log(K_{i^{\ast},t}^2/\eta^2)}{K_{i^{\ast},t}}} $, each with probability of at least $1 -  \frac{\pi^2}{6}\eta^2$. Hence with probability $1 - 2 \frac{\pi^2}{6}\eta^2$, we have %$(1 - \eta^2 \frac{\pi^2}{6})^2$, 
\begin{align}
\mu_i + \sqrt{\frac{2\log(K_{i,t}^2/\eta^2)}{K_{i,t}}} + \frac{\rho_i}{K_{i,t}} \geq \mu_{i^{\ast}}\,. \notag
\end{align}
When arm $i$ is pulled, arm $i$ wants to ensure the following holds
\begin{align}
 \sqrt{\frac{2\log(K_{i,t}^2/\eta^2)}{K_{i,t}}} + \frac{\rho_i}{K_{i,t}} \geq \delta_i\,,\notag
\end{align}
where $\delta_i = \mu_{i^{\ast}} - \mu_i$. Then,
\begin{equation*}
B_i \geq \rho_i \geq \left(\delta_i - \sqrt{\frac{2\log(K_{i,t}^2/\eta^2)}{K_{i,t}}}\right) \cdot K_{i,t}\,. \qedhere
\end{equation*}
\end{proof}

\section{Collusion strategy with the objective of regret maximization}
Stemming from the strong correlation between the cumulative regret and the number of suboptimal pulls, the optimal collusion strategy under the regret maximization objective is a variant of the combinatorial optimization problem defined earlier. Specifically, the maximization objective of the optimization problem takes a priority weight of each $Y_i$ based on the $\delta_i = \mu_i - \mu_{i^\ast}$, as
\begin{equation*}
\begin{aligned}
& \underset{Y_{i},t_i,\ i\in [m]}{\mathrm{maximize}}
& & \delta_1 \cdot Y_{1}+\dots+ \delta_m \cdot Y_{m} \\
& \mathrm{subject}\text{ }\mathrm{to}
& & \frac{B_i}{Y_{i}} + \sqrt{\frac{3\log t_i}{Y_{i}}} \ge \delta_i + \sqrt{3\log t_i},\ i \in [m]\,, \\
& & &  t_{i_j} \ge \sum_{l=1}^j Y_{i_l}, \ j\in [m]\,,\\
& & &  \textup{for some permutation}\ i_1,\dots\ i_m\ \textup{of}\ [m]\,.\\
\end{aligned}
\end{equation*}

\section{Additional simulation results}
\begin{figure*}[htbp]
\centering
\subfigure[]{
\label{Fig7}
\includegraphics[width=8cm,height=6cm,keepaspectratio]{figs/diff_B_card4.png}}
\subfigure[]{
\label{Fig8}
\includegraphics[width=8cm,height=6cm,keepaspectratio]{figs/diff_scale.png}}
\caption{\ref{Fig7} Cumulative regret v.s. time horizon with different level of strategic budget; \ref{Fig8} Effects of tuning UCB exploration parameter.}
\end{figure*}

\begin{figure*}[htbp]
\centering
\subfigure[]{
\label{Fig9}
\includegraphics[width=8cm,height=6cm,keepaspectratio]{figs/diff_arm_1010.png}}
\subfigure[]{
\label{Fig10}
\includegraphics[width=8cm,height=6cm,keepaspectratio]{figs/diff_arm_100.png}}
\caption{\ref{Fig9} Cumulative regret v.s. time horizon with different number of arms in each arm subset under $B_{max} = 10$; \ref{Fig10} Cumulative regret v.s. time horizon with different number of arms in each arm subset under $B_{max} = 100$.}
\end{figure*}
\begin{figure*}[htbp]
\centering
\subfigure[]{
\label{Fig5}
\includegraphics[width=8cm,height=6cm,keepaspectratio]{figs/pulls_final_final.png}}
\subfigure[]{
\label{Fig6}
\includegraphics[width=8cm,height=6cm,keepaspectratio]{figs/regret_final_final.png}}
\caption{\ref{Fig5} The number of suboptimal pulls v.s. collusion strategies; \ref{Fig6} Regret v.s. collusion strategies}
\end{figure*}
\bigbreak 

\paragraph{Experiment setting} All of the experiment settings remain the same as the experiments section unless otherwise indicated. 

\paragraph{Cumulative regret v.s. maximum budget} We experiment with $B_{max} = \{0, 10, 50, 100\}$ and $\gamma$ = $0.2$. Previously we have empirically evaluated the performance of strategic CUCB when each suboptimal arm process the same amount of strategic budget in Figure \ref{Fig1}. We now simulate the situation when suboptimal arms have strategic budgets of different levels by uniformly randomly assigning budgets from $[0,B_{max}]$ to each suboptimal arm. As shown in Figure \ref{Fig7}, the performance of strategic CUCB is still robust when there is a diversity of strategic budget owned by arms. Meanwhile, our strategic CUCB algorithm still outperforms naive CUCB under this scenario. 

\paragraph{Effects of tuning UCB exploration parameter} As shown in Figure \ref{Fig8}, our strategic CUCB achieves the best performance with $\gamma = 0.2$. This determines the discount parameter used in the experiment section. 
%With larger scaling factors, i.e. $\gamma = 0.5$, naive CUCB can attain lower regret than strategic CUCB.

\paragraph{More experiments on arm subset size} Similar to the experiment section, we relax the number of arms in each arm subset from $2$ to $4$ and $6$. We choose naive CUCB with $4$ arms in each arm subset as a baseline. We experiment on $B_{max} \in \{10, 50, 100\}$, respectively. Figure \ref{Fig9} and Figure \ref{Fig10} showcase that our algorithm outperforms naive CUCB regardless of the number of arms in each arm subset under all budget values.

\paragraph{Performance of different collusion strategies}
We experiment with three collusion strategies that are variants of the lump sum investing (LSI) strategy, which is the dominant Nash equilibrium strategy for the subgame between strategic arms. The maximum budget is set to be $50$. In prioritized budget LSI (PB-LSI) strategy, each strategic arm $i$ spends $\delta_i = \mu_{i^{\ast}} - \mu_i$ in the initialization rounds and then spends the rest of their budget all at once by the order of the value of their strategic budget. The prioritized delta LSI (PD-LSI) and prioritized budget-delta LSI (PBD-LSI) operate in similar fashions, but strategic arms spend budget according to the increasing order of their suboptimality gap $\delta_i = \mu_{i^{\ast}} - \mu_i$ and the increasing order of $B_i - \delta_i$, respectively. Figure \ref{Fig5} and Figure \ref{Fig6} showcase scenarios where the LSI strategy is suboptimal under the common objective of maximizing suboptimal pulls and maximizing regret. The figures show that considering the budget or suboptimal gap might not be sufficient for the decision of the collusion strategy, under both the objectives. It is clear that PBD-LSI outperforms the other three strategies. 
However, as the suboptimality gaps are constants, the effects of different collusion strategies on cumulative regret is limited and is fully observed in a short horizon.
